# Supplementary material for: Age-Invariant Face Embedding using the Wasserstein Distance
Source: arXiv:2305.02745 source file (2023-05-04)
Supplement: Supplementary file 1 [file arxiv-appendix-WMI-AI.pdf]

# Appendix: Age-Invariant Face Embedding using the Wasserstein Distance

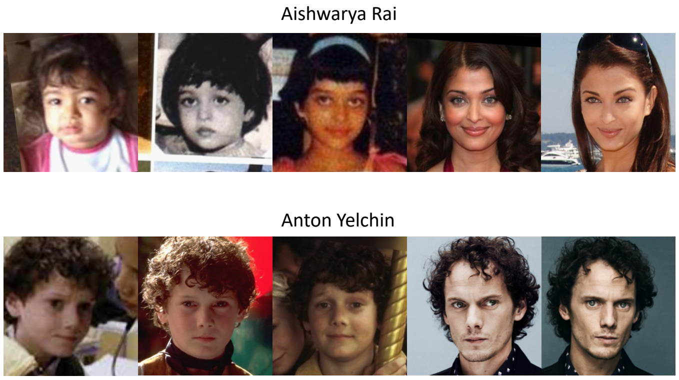


Fig. 1: From child to adult - the aging effect in face images. The images were taken from the ECAF dataset [2].

TABLE 1: The architecture of the age and identity classifiers, $\boldsymbol{g_a}$ and $\boldsymbol{g_{id}}$, respectively, detailed in Section 3.2, and the critic network of the discriminator $\boldsymbol{D}$ as in Section 3.1.

| $\boldsymbol{g_{id}}$ | $\boldsymbol{g_a}$ | $\boldsymbol{D}$ |
|---|---|---|
| Linear$(emb, D_{cls})$ | Linear$(emb, 101)$ | Linear$(emb \times 2, 150)$<br>LeakyRelu$(2 \cdot 10^{-1})$ |
| softmax | softmax | Linear$(150, 60)$<br>LeakyRelu$(2 \cdot 10^{-1})$ |
| ArcFace Loss[1] | CE Loss | Linear$(60, 20)$<br>LeakyRelu$(2 \cdot 10^{-1})$<br>Linear$(20, 1)$<br>BCE LOSS |

An ablation of the identity channel backbone and the critic network is reported in Table 2. For that, we used the MS1MV2 training dataset and set $\lambda_w = 0.1$. For the backbone of the identity CNN, we tested the ResNet and lightweight MobileNet networks. For the critic network, we tested a 3-layer MLP with outputs of $(60, 20, 1)$, while keeping the other settings fixed. The results in Table 2, show that using a shallower backbone for the identity CNN degrades the verification accuracy, while using a shallower critic network also reduces the verification accuracy, but to a lesser extent.

**Algorithm 1:** Training the WMI-AI age-invariant face embedding.

**Algorithm input** - face image $\boldsymbol{x}$, age label $\tau_a$, id label $\tau_{id}$.
**Initialize the encoders and classifiers** - $\boldsymbol{f_a}, \boldsymbol{f_{id}}, \boldsymbol{D}, \boldsymbol{g_a}, \boldsymbol{g_{id}}$
**Set hyperparameters** - $\lambda_w, \lambda_a, lr_w, lr$
**foreach** *epoch* **do**
  Randomly select a batch $\boldsymbol{x_i}$ of size $B$
  Compute $\boldsymbol{\hat{x}_{id}} = \boldsymbol{f_{id}(x_i)}$, $\boldsymbol{\hat{x}_a} = \boldsymbol{f_a(x_i)}$
  Set $\boldsymbol{\hat{x}} = (\boldsymbol{\hat{x}_a}, \boldsymbol{\hat{x}_{id}})$ ,$\boldsymbol{\bar{x}}, = (\psi(\boldsymbol{\hat{x}_a})\psi(\boldsymbol{\hat{x}_{id}}))$,$\psi$ is the shuffle operator
  **foreach** *step* $w$ **do**
    compute $L = L_w(\boldsymbol{\hat{x}}, \boldsymbol{\bar{x}}) - \lambda_g L_{grad}(\boldsymbol{\hat{x}}, \boldsymbol{\bar{x}})$
    backpropagate $D$ by maximizing $L$.
  **end foreach**
  Compute $L_w(\boldsymbol{\hat{x}}, \boldsymbol{\bar{x}})$
  Compute $\boldsymbol{g_a}(\boldsymbol{\hat{x}_a})$, $\boldsymbol{g_{id}}(\boldsymbol{\hat{x}_{id}})$
  Compute $L_a(\boldsymbol{g_a}, \tau_a, )$, $L_{id}(\boldsymbol{g_{id}}, \tau_{id})$
  backpropagate $\boldsymbol{g_{id}}$,$\boldsymbol{f_{id}}$ by minimizing $L_{id} + \lambda_w L_w$
  backpropagation $\boldsymbol{g_a}$,$\boldsymbol{f_a}$ by minimizing $\lambda_a L_a$
**end foreach**

## References

[1] Jiankang Deng, Jia Guo, Xue Niannan, and Stefanos Zafeiriou. ArcFace: additive angular margin loss for deep face recognition. In *Proceedings of the IEEE Conference on Computer Vision and Pattern Recognition (CVPR)*, 2019.

[2] Zhizhong Huang, Junping Zhang, and Hongming Shan. When age-invariant face recognition meets face age synthesis: A multi-task learning framework. In *Proceedings of the IEEE Conference on Computer Vision and Pattern Recognition (CVPR)*, 2021.

TABLE 2: Ablation of the backbone of the identity network and the critic networks. We report the verification accuracy [%] results.

| Method | CALFW | AgeDB30 | CACD-VS | ECAF(A,C) | ECAF(C,C) |
|---|---|---|---|---|---|
| WMI-AI+Resnet50 | 96.23 | 98.25 | **99.57** | 90.28 | 93.6 |
| WMI-AI+Resnet34 | 96.13 | 98.1 | 99.55 | 89.98 | 93.3 |
| WMI-AI+MobileNet | 95.69 | 97.18 | 99.5 | 88.26 | 90.85 |
| WMI-AI+smaller critic network | 96.23 | 98.29 | 99.55 | 90.57 | 94.05 |
| WMI-AI | **96.26** | **98.37** | **99.57** | **90.73** | **94.40** |
